# Supplementary material for: LEROjD: Lidar Extended Radar-Only Object Detection
Source: arXiv:2409.05564 source file (2024-09-09)
Supplement: Supplementary file 1 [file 12_appendix.tex]

\section{Appendix Section}
Supplementary material goes here.

% - Gegenüberstellung der beiden Sensoren Parameter. 
